# Supplementary material for: Sim-to-Real Learning of Footstep-Constrained Bipedal Dynamic Walking
Source: arXiv:2203.07589 source file (2022-05-03)
Supplement: Supplementary file 1 [file appendix.tex]

% !TEX root =  main.tex
% \section{APPENDIX}
\begin{appendix}
\begin{table}[!h]
\centering
\begin{tabular}{l|l}
\hline
Weight & Cost Component \\ \hline
0.155 &  Left foot force penalty \\ \hline
0.125 &  Right foot force penalty \\ \hline
0.155 &  Left foot velocity penalty \\ \hline
0.125 &  Right foot velocity penalty \\ \hline
0.125 &  Pelvis rate of change \\ \hline
0.125 &  Orientation penalty \\ \hline
0.125 &  Pelvis stabilization penalty \\ \hline
0.0325 & Action smoothness \\ \hline  
0.0325 & Torque penalty \\ \hline
3 & Footstep target (sparse) \\ \hline
\end{tabular}
\caption{Reward breakdown. \helei{need a compact way to say the basic reward terms, removing the speed tracking, adding pelvis movement and step sparse, without complicating too much}
}
\label{table:reward}
\end{table}
\end{appendix}
